# Supplementary material for: Spatial Optimization of Interconnected Systems in Non-Convex Design Spaces
Source: arXiv:2605.17387 source file (2026-05-17)
Supplement: Supplementary file 1 [file Appendix_Z.tex]

\begin{table}[h!]
\centering
\caption{Variables and notation (ordered by symbol) — Part 1}
\footnotesize
\setlength{\tabcolsep}{5pt}

\begin{tabularx}{\columnwidth}{@{}l l X@{}}
\textbf{Symbol} & \textbf{Type} & \textbf{Meaning / Range} \\
\hline
\(A_i\) & set & Object \(i\) represented as a set of spheres: \(A_i=\{b_{i,1},\dots,b_{i,n_{\mathrm{b},i}}\}\). \\
\(\mathcal{C}\) & set & Checked routing–routing segment-pair set defined in~\eqref{eq:SetS}. \\
\(\mathbb{F}_{A_i}\) & frame & Object frame attached to \(A_i\). \\
\(\mathbb{F}_\mathbb{W}\) & frame & Cartesian frame attached to \(\mathbb{W}\). \\
\(K_L\) & int & Number of segments in route \(L\) (\(K_L=n_{\mathrm{cp},L}+1\)). \\
\(L\) & index & Route index. \\
\(N_{\mathrm{pairs}}\) & int & Number of sphere–pair constraints across all objects. \\
\(N_{\mathrm{r\mbox{-}o}}\) & int & Number of routing–object interference constraints. \\
\(N_{\mathrm{r\mbox{-}r}}\) & int & Number of routing–routing interference constraints (\(|\mathcal{C}|\)). \\
\(S_{\alpha}(\cdot)\) & operator & Boltzmann (soft) operator; smooth approx. of \(\max/\min\) depending on sign of \(\alpha\). \\
\(\mathbb{W}\) & set & Workspace in \(\mathbb{R}^{n_\mathrm{d}}\). \\
\(\alpha\) & scalar & Soft-operator sharpness parameter. \\
\(b_{i,\mu}\) & sphere & Sphere \(\mu\) of object \(i\). \\
\(\mathbf{c}_{L,k}\) & vector \(\in\mathbb{R}^3\) & Control point \(k\) of route \(L\). \\
\(d^{\,\mathrm{obj\mbox{-}obj}}_{i,\mu,j,\nu}\) & scalar & Clearance between spheres \(b_{i,\mu}\) and \(b_{j,\nu}\) (Eq.~\eqref{eq:clearance_objobj}). \\
\(d^{\,\mathrm{route\mbox{-}obj}}_{L,m,i,\mu}\) & scalar & Clearance between routing segment \((L,m)\) and sphere \(b_{i,\mu}\). \\
\(d^{\,\mathrm{route\mbox{-}route}}_{L,m,L',\eta}\) & scalar & Clearance between routing segments \((L,m)\) and \((L',\eta)\). \\
\(f_\mathrm{re}\) & scalar & Exponential routing-length objective. \\
\(f_\mathrm{rq}\) & scalar & Squared routing-length objective \eqref{eq:frl}. \\
\(f_\mathrm{v}\) & scalar & AABB volume using objects only. \\
\(f_\mathrm{vr}\) & scalar & AABB volume using objects and routing points. \\
\(\mathbf{g}^{\mathrm{obj\mbox{-}obj}}\) & vector & Stacked object–object non-overlap constraints. \\
\(\mathbf{g}^{\mathrm{route\mbox{-}obj}}\) & vector & Stacked routing–object non-overlap constraints. \\
\end{tabularx}
\end{table}

\begin{table}[h!]
\centering
\caption{Variables and notation (ordered by symbol) — Part 2}
\footnotesize
\setlength{\tabcolsep}{5pt}

\begin{tabularx}{\columnwidth}{@{}l l X@{}}
\textbf{Symbol} & \textbf{Type} & \textbf{Meaning / Range} \\
\hline
\(\mathbf{g}^{\mathrm{route\mbox{-}route}}\) & vector & Stacked routing–routing non-overlap constraints. \\
\(g_\mathrm{soft}^{\mathrm{obj\mbox{-}obj}}\) & scalar & Soft aggregate of \(\mathbf{g}^{\mathrm{obj\mbox{-}obj}}\). \\
\(g_\mathrm{soft}^{\mathrm{route\mbox{-}obj}}\) & scalar & Soft aggregate of \(\mathbf{g}^{\mathrm{route\mbox{-}obj}}\). \\
\(g_\mathrm{soft}^{\mathrm{route\mbox{-}route}}\) & scalar & Soft aggregate of \(\mathbf{g}^{\mathrm{route\mbox{-}route}}\). \\
\(i,j\) & indices & Object indices (\(1\le i<j\le n_\mathrm{obj}\)). \\
\(k\) & index & Control-point index. \\
\(\ell\) & index & Port index on object \(i\) (\(1,\dots,n_{\varphi,i}\)). \\
\(m,\eta\) & indices & Routing segment indices. \\
\(n_\mathrm{d}\) & int & Workspace dimension (here \(=3\)). \\
\(n_\mathrm{obj}\) & int & Number of rigid objects. \\
\(n_{\mathrm{b},i}\) & int & Number of spheres representing object \(i\). \\
\(n_{\mathrm{cp},L}\) & int & Number of control points of route \(L\). \\
\(n_\mathrm{prob}\) & int & Problem index in \(\{1,2,3,4\}\). \\
\(n_\mathrm{var}\) & int & Total number of design variables \(=6(n_\mathrm{obj}-1)+3\sum_L n_{\mathrm{cp},L}\). \\
\(\mathbf{p}^{A_i}\) & vector \(\in\mathbb{R}^3\) & Point expressed in object frame \(\mathbb{F}_{A_i}\). \\
\(\mathbf{p}^{\mathbb{W}}\) & vector \(\in\mathbb{R}^3\) & Transformed point in workspace frame \(\mathbb{F}_\mathbb{W}\). \\
\(\mathbf{p}^{\mathbb{W}}_{\mathrm{b}_{i,\mu}}\) & vector \(\in\mathbb{R}^3\) & Center of sphere \(b_{i,\mu}\) in workspace frame. \\
\(\mathbf{p}_{\mathrm{proj},L,m}\) & vector \(\in\mathbb{R}^3\) & Closest point on routing segment \((L,m)\) to a given sphere center. \\
\(\mathbf{q}_{L,k}\) & vector \(\in\mathbb{R}^3\) & Route node: start/end port or control point. \\
\(r_{\mathrm{b}_{i,\mu}}\) & scalar & Radius of sphere \(b_{i,\mu}\). \\
\(r_r\) & scalar & Routing-tube radius. \\
\(\mathbf{R}_i\) & matrix \(\in\mathbb{R}^{3\times 3}\) & Rotation from \(\mathbb{F}_{A_i}\) to \(\mathbb{F}_\mathbb{W}\) (RPY composition). \\
\(\mathbf{t}_i\) & vector \(\in\mathbb{R}^3\) & Translation of object \(i\) in \(\mathbb{F}_\mathbb{W}\). \\
\(\varphi_{i,\ell}\) & point & Port \(\ell\) on object \(i\). \\
\(w_\mathrm{v},w_\mathrm{vr},w_\mathrm{rq},w_\mathrm{re}\) & scalars & Weights for the objective functions. \\
\(\mathbf{x}\) & vector & Stacked design variables \([\mathbf{x}_2^\top,\dots,\mathbf{x}_{n_\mathrm{obj}}^\top,\mathbf{c}_{1,1}^\top,\dots]^\top\). \\
\(\mathbf{x}_{\mathrm{o}i}\) & vector \(\in\mathbb{R}^6\) & Pose of object \(i\): RPY \((x_{\theta,i},x_{\alpha,i},x_{\beta,i})\) and translation \((x_{x,i},x_{y,i},x_{z,i})\). \\
\(\mu,\nu\) & indices & Sphere indices for objects \(i\) and \(j\). \\
\end{tabularx}
\end{table}
\endgroup
